# Supplementary material for: MG-GAN: A Multi-Generator Model Preventing Out-of-Distribution Samples in Pedestrian Trajectory Prediction
Source: arXiv:2108.09274 source file (2021-08-20)
Supplement: Supplementary file 1 [file biwi_num_gens.tex]

\begin{tabular}{lrrrr}
\toprule
\# Generators &          2 &          3 &          4 &          5 \\
Dataset &            &            &            &            \\
\midrule
ETH     &  0.47/0.92 &  0.52/1.00 &  0.52/0.99 &  0.58/1.10 \\
HOTEL   &  0.14/0.24 &  0.15/0.27 &  0.16/0.30 &  0.15/0.27 \\
UNIV    &  0.56/1.11 &  0.54/1.07 &  0.56/1.10 &  0.55/1.09 \\
ZARA1   &  0.36/0.73 &  0.36/0.73 &  0.37/0.75 &  0.37/0.75 \\
ZARA2   &  0.29/0.60 &  0.30/0.62 &  0.30/0.61 &  0.29/0.61 \\
\midrule
AVG     &  0.37/0.72 &  0.38/0.74 &  0.38/0.75 &  0.39/0.76 \\
\bottomrule
\end{tabular}
